# Supplementary material for: Counting and Computing Join-Endomorphisms in Lattices (Revisited)
Source: arXiv:2211.00781 source file (2022-11-01)
Supplement: Supplementary file 1 [file appendix-sec-proofs-algo.tex]

% !TeX root = ../main.tex

\section{Proofs}
\label{sec:proofs}

% !TeX root = ../main.tex

\subsection{Proof of Theorem~\ref{size4m-n:lemma}.}
\label{app:proof-count-Mn}

We shall show that $|\sfunspace{\M_n}|$ can be expressed in terms of Laguerre polynomials:
\( |\sfunspace{\M_n}| = (n+1)^2  +  n! \laguerre{n}{-1}\).

Let $\fcal = \bigcup_{i=1}^4\fcal_i$ where the mutually exclusive $\fcal_i$'s
are defined in Table~\ref{sfunc-mn-red:table}, and $I=\{1,\ldots,n\}$. The proof is divided in two parts: (I) $\sfunspace{\M_n} = \fcal$
and (II) $|\fcal| = (n+1)^2  +  n! \laguerre{n}{-1}.$

\subsubsection{Part (I)} For $\fcal \subseteq \sfunspace{\M_n}$, it is easy to verify that each $f \in \fcal$ is a join-endomorphism.

For $\sfunspace{\M_n} \subseteq \fcal$ we show that for any function $f$ from $\M_n$ to $\M_n$  if $f \not\in \fcal$, then $f \not\in \sfunspace{\M_n}$. Immediately, if $f(\bot)\neq \bot$ then $f \not\in  \sfunspace{\M_n}$. 

Suppose $f(\bot) = \bot$.
Let $J, K, H$ be disjoint possibly empty sets such that $I = J \cup K \cup H$ and
let $j= |J|$, $k = |K|$ and $h = |H|$. The sets $J, K, H$ represent the elements of $I$ mapped by $f$ to $\top$,  
to elements of $I$, and to $\bot$, resp. More precisely,
$\mathrm{Img}(\fres{f}{J}) = \{\top\}$,
$\mathrm{Img}(\fres{f}{K}) \subseteq I$ and
$\mathrm{Img}(\fres{f}{H}) = \{\bot\}$.
Furthermore, for every $f$ either (1) $f(\top) = \bot$, (2) $f(\top) \in I$ or (3) $f(\top) = \top$. For each case we show that $f \not\in  \sfunspace{\M_n}$. 

\begin{enumerate}
\item $f(\top) = \bot$. Since $f \not\in \fcal_1$ there is an $e \in I$ such that $f(e) \neq \bot$. We have $e \cleq \top$ but $f(e) \not\cleq f(\top)$. Then $f$ is not monotonic.
From Prop. \ref{prop:monotonicity} we conclude  $f \not\in \sfunspace{\M_n}$.

\item $f(\top) \in I$. Let $K_1,K_2$ be disjoint possibly empty sets such that $K_1 \cup K_2 = K$,
$\mathrm{Img}(\fres{f}{K_1}) = \{f(\top)\}$ and
$\mathrm{Img}(\fres{f}{K_2}) \neq \{f(\top)\}$.
Notice that if $j > 0$ or $|K_2| > 0$, $f$ is non-monotonic and then
$f \not\in \sfunspace{\M_n}$.

We then must have $j = 0$ and $K_2 = \emptyset$. Since $\mathrm{Img}(\fres{f}{K})
= \{f(\top)\}$ and $f \not\in \fcal_2$ then $h > 1$. Therefore there must be
$e_1, e_2 \in H$ such that $f(e_1) = f(e_2) = \bot$. This implies
$f(e_1 \join e_2) = f(\top) \neq \bot = f(e_1) \join f(e_2)$, therefore $f \not\in \sfunspace{\M_n}$.

\item $f(\top) = \top$. 

\begin{enumerate}[label*=\arabic*.]
\item Suppose $k = 0$. Notice that $f \not\in \fcal_3$ and $f \not\in \fcal_4$
hence $h \neq 1$ and $h \neq 0$. Thus $h >1$ implies that
there are at least two $e_1, e_2 \in H$ such that $f(e_1) = f(e_2) = \bot.$
But then  $f(e_1 \join e_2) = f(\top) = \top \neq \bot = f(e_1) \join f(e_2)$,
hence $f \not\in \sfunspace{\M_n}$.

\item Suppose $k > 0$.
Assume $h=0.$ Let $K_1, K_2$ be disjoint possibly empty sets
such that $K_1 \cup K_2 = K$, $\mathrm{Img}(\fres{f}{K_1}) \subseteq J$ 
and $\mathrm{Img}(\fres{f}{K_2}) \subseteq I \setminus J$. 
Notice that $f$ is a  $\bot$ and $\top$ preserving function and satisfies conditions (a) and (c)
of $\fcal_4$ but   $f \not\in \fcal_4$, then $f$ must violate condition (b). Thus $\fres{f}{K_1}$ or
$\fres{f}{K_2}$ is not injective. Let us assume that  $\fres{f}{K_1}$ is not injective (the case when 
$\fres{f}{K_2}$
is not injective is analogous). 
Then there are $a,b \in K_1$ and $c \in J$, such that
$a \neq b$ but $f(a) = f(b) = c$. By definition
$\top \not\in J$, then $f(a) \join f(b) = c \neq \top = f(a \join b)$. Consequently, $f \not\in \sfunspace{\M_n}$.

Assume $h>0$. There must be $e_1, e_2, e_3 \in I$  such that $f(e_1) = \bot$
and $f(e_2) = e_3$. Notice $e_1 \join e_2 = \top$, we then have 
$f(e_1) \join f(e_2) = e_3 \neq \top = f(e_1 \join e_2)$. Therefore, 
$f \not\in \sfunspace{\M_n}$.
\end{enumerate} 

% Since $f \not\in \fcal_2$, from condition (b) we know that for all
% $e_1,e_2 \in I$, $f(e_1) \neq \bot$ and $f(e_2) \neq e_1$.
% Taking $e_1 = e$ and $e_2 = e'$, we have $f(e) \neq \bot$ and
% $f(e') \neq e$. Notice that $f(e \join \top) = e'$ and
% $f(e) \join f(\top) = f(e) \join e'$, where $f(e) \neq e'$ and
% $f(e) \neq \bot$. Then $f(e) \join e' = \top$ and $f(e \join \top)
% \neq f(e) \join f(\top)$. Therefore $f \not\in \sfunspace{\M_n}$.

\end{enumerate}

\subsubsection{Part (II)} We prove that $|\fcal| = \sum_{i=1}^4|\fcal_i| = (n+1)^2  +  n! \laguerre{n}{-1}$.
Recall that $n = |I|$.

\begin{enumerate}
\item $|\fcal_1| = 1$.
There is only one function mapping every element in $\M_n$ to $\bot$.

\item $|\fcal_2| = n^2 + n$.
Since $\top$ is mapped to an element of $I$, there are $n$ 
possibilities to choose such element. If there is an element of $I$ mapped to
$\bot$, for each one of the previous $n$ options there are also $n$
possibilities to choose an element of $I$ to be mapped to $\bot$.
Then, in this case there are $n^2$ functions. If no element of $I$
is mapped to $\bot$, then there are $n$ additional functions.

\item $|\fcal_3| = n$. One of the elements of $I$ is mapped to $\bot$.
All the other elements of $I$ are mapped to $\top$. Then, there are $n$ 
functions that can be defined in $\fcal_3$.

\item $|\fcal_4| = \Rook{n}{1}$.
Let $f \in \fcal_4$ and let $J, K_1, K_2$ be disjoint possibly empty sets 
such that $I = J \cup K_1 \cup K_2$,
$\mathrm{Img}(\fres{f}{J}) = \{\top\}$,
$\mathrm{Img}(\fres{f}{K_1}) \subseteq J$ and
$\mathrm{Img}(\fres{f}{K_2}) \subseteq I \setminus J$, where
$\fres{f}{K_1}$ and $\fres{f}{K_2}$ are injective functions.
We shall call $j = |J|$ and $k_1 = |K_1|$.
% Note that $|K_2| = n-j-k_1$.

%Now, there are $\binom{n}{j}$ possibilities to choose $J$ among the 
%elements of $I$. For each choice of $J$, the elements of $K_1$ are to be 
%mapped to elements of $J$ by the injective function $\fres{f}{K_1}$.
%This is possible only if $k_1\leq j$, then we take $k_1 \leq \min(j,n-j)$.
%The number of choices of $K_1$ is $\binom{n-j}{k_1}$ and the number of choices
%among $J$ that can be targets of the elements of $K_1$ is $\binom{j}{k_1}$.
%Each of this can be targeted by any permutation of $K_1$, then we have 
%$\binom{j}{k_1}k_1! = \frac{j!}{(j-k_1)!}$ possibilities to choose $K_1$
%and map its elements by $\fres{f}{K_1}$ to elements of $J$. Similarly,
%the number of possibilities to choose $K_2$ and map its elements
%by $\fres{f}{K_2}$ to elements of $I \setminus J$ is
%$\binom{n-j}{n-j-k_1}(n-j-k_1)! = \frac{(n-j)!}{k_1!}$.
%Therefore, $|\fcal_4| = \sum_{j=0}^{n}\binom{n}{j} \sum_{k_1=0}^{\min(j,n-j)}
%\binom{n-j}{k_1}\frac{j!}{(j-k_1)!}\frac{(n-j)!}{k_1!}$.

For each of the $\binom{n}{j}$ possibilities  for $J$, the elements of $K_1$ are to be 
mapped to them by the injective function $\fres{f}{K_1}$.
This is possible only if $k_1\leq j$, so we take $k_1 \leq \min(j,n-j)$.
The number of choices of $K_1$ is $\binom{n-j}{k_1}$ and the number of choices
among $J$ that can be targets of those is $\binom{j}{k_1}$.
Each of these can be mapped from any permutation of $K_1$, so we have 
$\binom{j}{k_1}k_1! = \frac{j!}{(j-k_1)!}$ possibilities to choose $K_1$
and map its elements by $\fres{f}{K_1}$ to elements of $J$. Similarly,
the number of possibilities to choose $K_2$ and map its elements
by $\fres{f}{K_2}$ to elements of $I \setminus J$ is
$\binom{n-j}{n-j-k_1}(n-j-k_1)! = \frac{(n-j)!}{k_1!}$.
Therefore, $|\fcal_4| = \sum_{j=0}^{n}\binom{n}{j} \sum_{k_1=0}^{\min(j,n-j)}
\binom{n-j}{k_1}\frac{j!}{(j-k_1)!}\frac{(n-j)!}{k_1!}$.
We can simplify the inner sum:
\( \sum_{k_1=0}^{\min(j,n-j)} \binom{n-j}{k_1}\frac{j!}{(j-k_1)!}\frac{(n-j)!}{k_1!}
= \frac{n!}{j!}\).
We then obtain  $|\fcal_4| = \sum_{j=0}^{n}\binom{n}{j}
\frac{n!}{j!}$. This sum equals $n!\laguerre{n}{-1}$ which in turn 
is equal  to $\Rook{n}{1}.$

\end{enumerate}

It follows that $|\fcal| = \sum_{i=1}^4|\fcal_i| = (n + 1)^2 + n! \laguerre{n}{-1} $ as wanted. 
\qed

% \subsubsection{Proof of Theorem~\ref{rook:th}.}
% We wish to prove that $| A | = \Rook{n}{1}$ where $ A=  \{ \ f \in \sfunspace{\M_n} \mid f \mbox{ is non-reducing in }  \M_n \ \} $. Let $\fcal = \bigcup_{i=1}^4\fcal_i$ where the mutually exclusive $\fcal_i$'s
% are defined in Table~\ref{sfunc-mn-red:table}. In the proof of Theorem~\ref{size4m-n:lemma} we show that $\sfunspace{\M_n} = \fcal$ and that  $\Rook{n}{1} = |\fcal_4|$.  Notice that every function in $\fcal_4$ is non-reducing and every function in $\fcal \setminus \fcal_4$ is not non-reducing. Hence $A = \fcal_4$, thus $ | A | = \Rook{n}{1}.$

% \input{\mainDir/Body/subsec-proof-lemma4-sergio}

% \input{\mainDir/Body/subsec-proof-thm2-sergio}

% \input{\mainDir/Body/subsec-proof-thm-camilo}
